# Supplementary material for: On Stochastic Estimation of Partition Function
Source: arXiv:1401.7273 source file (2014-01-28)
Supplement: Supplementary file 1 [file appendix.tex]

\appendix
This section contains temporary elaborations that may or may not make it to the final paper.
\section{}
\subsection{Delta Method}
Let $X$ be a RV with distribution $p_{X}$, mean $\mu$ and variance $\sigma^{2}$, and let
$Y:=f(X)$ for some function $f$. 
Using Taylor expansion around $\mu$, the first order approximation of $Y$  
\[
Y \simeq f(\mu) + (X-\mu)f'(\mu),
\]
where $f'(\mu):={df}/{dx}|_{x=\mu}$.
Then,
$E[Y] = f(\mu)$ and $\var[Y] = f'(\mu)^{2}$.
Clearly, the approximation is inaccurate for the case of interest where $f$ is a nonlinear function, unless if
$X$ is a degenerate RV, i.e., $p_{X}$ has all its mass centered at one point. This is exactly the situation where this
method is useful, namely when there is an estimator $X$ that converges to its mean, and one is interested in the variance
of another estimator $Y = f(X)$. This method is called the ``delta method.'' 

In our case, 
\[X:=\frac{1}{M} \sum\limits_{i=1}^{M}\frac{1}{f_{\G}(X_{i})},\]
where $X_{1}, \cdots, X_M$ are independently drawn from the NFG distribution $p_{\G}:=f_{\G}/Z_{\G}$, and $f(X) =
\frac{|\X_{\G}|}{X}$.
Hence,
$f'(X) = -|\X_{\G}|/X^{2}$,
and
$\mu$ converges to $E[1/f_{\G}(X_{1})] = |\X_{\G}|/Z_{\G}$ for large $M$, and so
\begin{eqnarray*}
	\var\big[\frac{1}{X}\big] \hspace{-.6cm}
	&&= \frac{|\X_{\G}|^2}{\mu^{4}} \var[X] = \frac{Z_{\G}^{4}}{|\X_{\G}|^2} \var[X] \\
	&&= \frac{Z_{\G}^{4}}{M|\X_{\G}|^2} \var[\frac{1}{f_{\G}(X_1)}] 
\end{eqnarray*}

\subsection{Dual NFG for the clock model}
Given $f(x):=e^{\beta \cos(2\pi x/q)}$ for all $x \in \Z_{q}$, we show that $\widehat{f}(\hat{x}) \geq 0$ for all
$\hat{x} \in \widehat{\Z_{q}}$.
Using Taylor expansion, we have
\[
f(x) = \sum_{n=0}^{\infty} \frac{\beta^{n}g_{n}(x)}{n!},
\]
where 
\begin{eqnarray*}
	g_{n}(x)\hspace{-.6cm}&&
	:=\cos^{n}(2\pi x/q) 
	=\frac{1}{2^{n}}\big(\chi_{1}(x)+\chi_{1}(-x)\big)^{n} \\
	&&= \frac{1}{2^{n}}\sum_{l=0}^{n} \binom{n}{l} \chi_{1}^{n-l}(x) \chi_{1}^{l}(-x)  \\
	&&= \frac{1}{2^{n}}\sum_{l=0}^{n} \binom{n}{l} \chi_{n-2l}(x).
\end{eqnarray*}
Hence,
\[
\widehat{g_{n}}(\chi_{k}) = \frac{q}{2^{n}}\sum_{l=0}^{n}\binom{n}{l}[n+k-2l = 0]
\]
 is a non-negative function that is upper bounded by $q$,
and so
\[
\widehat{f}(\chi_{k}) = \sum_{n=0}^{\infty} \frac{\beta^{n}\widehat{g_{n}}(\chi_{k})}{n!}
\]
is also a non-negative function, 
where the series is convergent since
\[
\sum_{n=0}^{\infty} \frac{\beta^{n}\widehat{g_{n}}(\chi_{k})}{n!}
\leq q\sum_{n=0}^{\infty} \frac{\beta^{n}}{n!} = q e^{\beta}.
\]
%\[0 \leq \lim\limits_{n\rightarrow \infty} \frac{\beta^{n}\widehat{g_{n}}}{n!}\leq \lim\limits_{n\rightarrow \infty}
%\frac{\beta^{n}q}{n!}\ =0.\]
